# Supplementary material for: MANTRA: The Manifold Triangulations Assemblage
Source: arXiv:2410.02392 source file (2025-03-03)
Supplement: Supplementary file 1 [file appendix_betti_accuracy_full_stage.tex]

\begin{tabular}{lllllllllllllll}
	{}                         & {}                              & {metric}    & \multicolumn{12}{c}{Accuracy}                                                                                                                                                                                                                                                                                                    \\
	{}                         & {}                              & {task}      & \multicolumn{3}{c}{Betti 0}   & \multicolumn{3}{c}{Betti 1} & \multicolumn{3}{c}{Betti 2} & \multicolumn{3}{c}{Betti 3}                                                                                                                                                                                                          \\
	{}                         & {}                              & {transform} & {Degree Transform}            & {Degree Transform Onehot}   & {Random Node Features}      & {Degree Transform}          & {Degree Transform Onehot} & {Random Node Features} & {Degree Transform} & {Degree Transform Onehot} & {Random Node Features} & {Degree Transform} & {Degree Transform Onehot} & {Random Node Features} \\
	{dataset}                  & {modelclass}                    & {Model}     & {}                            & {}                          & {}                          & {}                          & {}                        & {}                     & {}                 & {}                        & {}                     & {}                 & {}                        & {}                     \\
	\multirow[c]{12}{*}{F2D0}  & \multirow[c]{5}{*}{Graph}       & GAT         & 1.0 \pm 0.0                   & 1.0 \pm 0.0                 & 1.0 \pm 0.0                 & 0.31 \pm 0.0                & 0.31 \pm 0.0              & 0.31 \pm 0.0           & 0.92 \pm 0.0       & 0.92 \pm 0.0              & 0.92 \pm 0.0           &                    &                           &                        \\
	                           &                                 & GCN         & 1.0 \pm 0.0                   & 1.0 \pm 0.0                 & 1.0 \pm 0.0                 & 0.31 \pm 0.0                & 0.31 \pm 0.0              & 0.31 \pm 0.0           & 0.92 \pm 0.0       & 0.92 \pm 0.0              & 0.92 \pm 0.0           &                    &                           &                        \\
	                           &                                 & MLP         & 1.0 \pm 0.0                   & 1.0 \pm 0.0                 & 1.0 \pm 0.0                 & 0.31 \pm 0.0                & 0.31 \pm 0.0              & 0.31 \pm 0.0           & 0.92 \pm 0.0       & 0.92 \pm 0.0              & 0.92 \pm 0.0           &                    &                           &                        \\
	                           &                                 & TAG         & 1.0 \pm 0.0                   & 1.0 \pm 0.0                 & 1.0 \pm 0.0                 & 0.32 \pm 0.01               & 0.33 \pm 0.01             & 0.32 \pm 0.0           & 0.92 \pm 0.0       & 0.92 \pm 0.0              & 0.92 \pm 0.0           &                    &                           &                        \\
	                           &                                 & TRANSFCONV  & 1.0 \pm 0.0                   & 1.0 \pm 0.0                 & 1.0 \pm 0.0                 & 0.33 \pm 0.0                & 0.32 \pm 0.01             & 0.32 \pm 0.01          & 0.92 \pm 0.0       & 0.92 \pm 0.0              & 0.92 \pm 0.0           &                    &                           &                        \\
	                           & \multirow[c]{7}{*}{Topological} & Cell Mp     & 0.46 \pm 0.5                  &                             & 1.0 \pm 0.0                 & 0.39 \pm 0.35               &                           & 0.9 \pm 0.01           & 0.46 \pm 0.44      &                           & 0.92 \pm 0.0           &                    &                           &                        \\
	                           &                                 & Cell Transf & 1.0 \pm 0.0                   &                             & 1.0 \pm 0.0                 & 0.93 \pm 0.0                &                           & 0.87 \pm 0.0           & 0.93 \pm 0.0       &                           & 0.92 \pm 0.0           &                    &                           &                        \\
	                           &                                 & DECT        & 1.0 \pm 0.0                   & 1.0 \pm 0.0                 & 1.0 \pm 0.0                 & 0.32 \pm 0.0                & 0.32 \pm 0.0              & 0.32 \pm 0.0           & 0.92 \pm 0.0       & 0.92 \pm 0.0              & 0.92 \pm 0.0           &                    &                           &                        \\
	                           &                                 & SAN         & 0.09 \pm 0.04                 &                             & 0.57 \pm 0.18               & 0.12 \pm 0.1                &                           & 0.54 \pm 0.11          & 0.52 \pm 0.14      &                           & 0.73 \pm 0.08          &                    &                           &                        \\
	                           &                                 & SCCN        & 1.0 \pm 0.0                   &                             & 0.71 \pm 0.06               & 0.93 \pm 0.0                &                           & 0.67 \pm 0.05          & 0.93 \pm 0.0       &                           & 0.79 \pm 0.04          &                    &                           &                        \\
	                           &                                 & SCCNN       & 0.0 \pm 0.0                   &                             & 0.01 \pm 0.0                & 0.03 \pm 0.02               &                           & 0.03 \pm 0.01          & 0.33 \pm 0.37      &                           & 0.49 \pm 0.12          &                    &                           &                        \\
	                           &                                 & SCN         & 0.33 \pm 0.38                 &                             & 0.29 \pm 0.07               & 0.21 \pm 0.26               &                           & 0.25 \pm 0.1           & 0.62 \pm 0.36      &                           & 0.65 \pm 0.08          &                    &                           &                        \\
	\multirow[c]{12}{*}{F3D0}  & \multirow[c]{5}{*}{Graph}       & GAT         & 1.0 \pm 0.0                   & 1.0 \pm 0.0                 & 1.0 \pm 0.0                 & 1.0 \pm 0.0                 & 1.0 \pm 0.0               & 1.0 \pm 0.0            & 1.0 \pm 0.0        & 1.0 \pm 0.0               & 1.0 \pm 0.0            & 1.0 \pm 0.0        & 1.0 \pm 0.0               & 1.0 \pm 0.0            \\
	                           &                                 & GCN         & 1.0 \pm 0.0                   & 1.0 \pm 0.0                 & 1.0 \pm 0.0                 & 1.0 \pm 0.0                 & 1.0 \pm 0.0               & 1.0 \pm 0.0            & 1.0 \pm 0.0        & 1.0 \pm 0.0               & 1.0 \pm 0.0            & 1.0 \pm 0.0        & 1.0 \pm 0.0               & 1.0 \pm 0.0            \\
	                           &                                 & MLP         & 1.0 \pm 0.0                   & 1.0 \pm 0.0                 & 1.0 \pm 0.0                 & 1.0 \pm 0.0                 & 1.0 \pm 0.0               & 1.0 \pm 0.0            & 1.0 \pm 0.0        & 1.0 \pm 0.0               & 1.0 \pm 0.0            & 1.0 \pm 0.0        & 1.0 \pm 0.0               & 1.0 \pm 0.0            \\
	                           &                                 & TAG         & 1.0 \pm 0.0                   & 1.0 \pm 0.0                 & 1.0 \pm 0.0                 & 1.0 \pm 0.0                 & 1.0 \pm 0.0               & 1.0 \pm 0.0            & 1.0 \pm 0.0        & 1.0 \pm 0.0               & 1.0 \pm 0.0            & 1.0 \pm 0.0        & 1.0 \pm 0.0               & 1.0 \pm 0.0            \\
	                           &                                 & TRANSFCONV  & 1.0 \pm 0.0                   & 1.0 \pm 0.0                 & 1.0 \pm 0.0                 & 1.0 \pm 0.0                 & 1.0 \pm 0.0               & 1.0 \pm 0.0            & 1.0 \pm 0.0        & 1.0 \pm 0.0               & 1.0 \pm 0.0            & 1.0 \pm 0.0        & 1.0 \pm 0.0               & 1.0 \pm 0.0            \\
	                           & \multirow[c]{7}{*}{Topological} & Cell Mp     & 1.0 \pm 0.0                   &                             & 1.0 \pm 0.0                 & 1.0 \pm 0.0                 &                           & 1.0 \pm 0.0            & 1.0 \pm 0.0        &                           & 1.0 \pm 0.0            & 1.0 \pm 0.0        &                           & 1.0 \pm 0.0            \\
	                           &                                 & Cell Transf & 1.0 \pm 0.0                   &                             & 1.0 \pm 0.0                 & 1.0 \pm 0.0                 &                           & 1.0 \pm 0.0            & 1.0 \pm 0.0        &                           & 1.0 \pm 0.0            & 1.0 \pm 0.0        &                           & 1.0 \pm 0.0            \\
	                           &                                 & DECT        & 1.0 \pm 0.0                   & 1.0 \pm 0.0                 & 1.0 \pm 0.0                 & 1.0 \pm 0.0                 & 1.0 \pm 0.0               & 1.0 \pm 0.0            & 1.0 \pm 0.0        & 1.0 \pm 0.0               & 1.0 \pm 0.0            & 1.0 \pm 0.0        & 1.0 \pm 0.0               & 1.0 \pm 0.0            \\
	                           &                                 & SAN         & 0.01 \pm 0.0                  &                             & 0.51 \pm 0.12               & 0.49 \pm 0.13               &                           & 0.71 \pm 0.11          & 0.51 \pm 0.22      &                           & 0.78 \pm 0.1           & 0.01 \pm 0.01      &                           & 0.52 \pm 0.07          \\
	                           &                                 & SCCN        & 1.0 \pm 0.0                   &                             & 1.0 \pm 0.0                 & 1.0 \pm 0.0                 &                           & 1.0 \pm 0.0            & 1.0 \pm 0.0        &                           & 1.0 \pm 0.0            & 1.0 \pm 0.0        &                           & 1.0 \pm 0.0            \\
	                           &                                 & SCCNN       & 0.0 \pm 0.0                   &                             & 0.0 \pm 0.0                 & 0.48 \pm 0.14               &                           & 0.48 \pm 0.05          & 0.6 \pm 0.08       &                           & 0.49 \pm 0.12          & 0.0 \pm 0.0        &                           & 0.0 \pm 0.0            \\
	                           &                                 & SCN         & 0.95 \pm 0.06                 &                             & 0.95 \pm 0.08               & 0.85 \pm 0.19               &                           & 0.99 \pm 0.01          & 0.8 \pm 0.16       &                           & 0.99 \pm 0.0           & 0.58 \pm 0.31      &                           & 0.92 \pm 0.08          \\
	\multirow[c]{12}{*}{NN2D0} & \multirow[c]{5}{*}{Graph}       & GAT         & 1.0 \pm 0.0                   & 1.0 \pm 0.0                 & 1.0 \pm 0.0                 & 0.54 \pm 0.0                & 0.54 \pm 0.0              & 0.54 \pm 0.0           & 0.7 \pm 0.0        & 0.7 \pm 0.0               & 0.7 \pm 0.0            &                    &                           &                        \\
	                           &                                 & GCN         & 1.0 \pm 0.0                   & 1.0 \pm 0.0                 & 1.0 \pm 0.0                 & 0.54 \pm 0.0                & 0.54 \pm 0.0              & 0.54 \pm 0.0           & 0.7 \pm 0.0        & 0.7 \pm 0.0               & 0.7 \pm 0.0            &                    &                           &                        \\
	                           &                                 & MLP         & 1.0 \pm 0.0                   & 1.0 \pm 0.0                 & 1.0 \pm 0.0                 & 0.54 \pm 0.0                & 0.54 \pm 0.0              & 0.54 \pm 0.0           & 0.7 \pm 0.0        & 0.7 \pm 0.0               & 0.7 \pm 0.0            &                    &                           &                        \\
	                           &                                 & TAG         & 1.0 \pm 0.0                   & 1.0 \pm 0.0                 & 1.0 \pm 0.0                 & 0.54 \pm 0.0                & 0.54 \pm 0.0              & 0.54 \pm 0.0           & 0.7 \pm 0.0        & 0.7 \pm 0.0               & 0.7 \pm 0.0            &                    &                           &                        \\
	                           &                                 & TRANSFCONV  & 1.0 \pm 0.0                   & 1.0 \pm 0.0                 & 1.0 \pm 0.0                 & 0.54 \pm 0.0                & 0.54 \pm 0.0              & 0.54 \pm 0.0           & 0.7 \pm 0.0        & 0.7 \pm 0.0               & 0.7 \pm 0.0            &                    &                           &                        \\
	                           & \multirow[c]{7}{*}{Topological} & Cell Mp     & 0.05 \pm 0.09                 &                             & 0.98 \pm 0.0                & 0.18 \pm 0.24               &                           & 0.65 \pm 0.01          & 0.14 \pm 0.31      &                           & 0.69 \pm 0.01          &                    &                           &                        \\
	                           &                                 & Cell Transf & 1.0 \pm 0.0                   &                             & 1.0 \pm 0.0                 & 0.36 \pm 0.06               &                           & 0.54 \pm 0.0           & 0.64 \pm 0.17      &                           & 0.7 \pm 0.01           &                    &                           &                        \\
	                           &                                 & DECT        & 1.0 \pm 0.0                   & 1.0 \pm 0.0                 & 1.0 \pm 0.0                 & 0.54 \pm 0.0                & 0.54 \pm 0.0              & 0.54 \pm 0.0           & 0.7 \pm 0.0        & 0.7 \pm 0.0               & 0.7 \pm 0.0            &                    &                           &                        \\
	                           &                                 & SAN         & 0.07 \pm 0.06                 &                             & 0.26 \pm 0.16               & 0.26 \pm 0.05               &                           & 0.26 \pm 0.11          & 0.43 \pm 0.09      &                           & 0.43 \pm 0.06          &                    &                           &                        \\
	                           &                                 & SCCN        & 1.0 \pm 0.0                   &                             & 0.48 \pm 0.03               & 0.69 \pm 0.03               &                           & 0.4 \pm 0.03           & 0.71 \pm 0.01      &                           & 0.52 \pm 0.01          &                    &                           &                        \\
	                           &                                 & SCCNN       & 0.0 \pm 0.0                   &                             & 0.01 \pm 0.0                & 0.08 \pm 0.1                &                           & 0.12 \pm 0.08          & 0.27 \pm 0.29      &                           & 0.35 \pm 0.08          &                    &                           &                        \\
	                           &                                 & SCN         & 0.01 \pm 0.02                 &                             & 0.13 \pm 0.03               & 0.2 \pm 0.01                &                           & 0.19 \pm 0.03          & 0.25 \pm 0.35      &                           & 0.43 \pm 0.03          &                    &                           &                        \\
	\multirow[c]{11}{*}{NN2D1} & \multirow[c]{5}{*}{Graph}       & GAT         & 0.0 \pm 0.0                   & 0.64 \pm 0.5                & 1.0 \pm 0.0                 & 0.2 \pm 0.0                 & 0.43 \pm 0.16             & 0.54 \pm 0.0           & 0.7 \pm 0.0        & 0.7 \pm 0.0               & 0.7 \pm 0.0            &                    &                           &                        \\
	                           &                                 & GCN         & 0.0 \pm 0.0                   & 0.68 \pm 0.46               & 1.0 \pm 0.0                 & 0.2 \pm 0.0                 & 0.47 \pm 0.15             & 0.54 \pm 0.0           & 0.7 \pm 0.0        & 0.7 \pm 0.0               & 0.7 \pm 0.0            &                    &                           &                        \\
	                           &                                 & MLP         & 0.53 \pm 0.49                 & 1.0 \pm 0.0                 & 1.0 \pm 0.0                 & 0.34 \pm 0.14               & 0.54 \pm 0.0              & 0.54 \pm 0.0           & 0.7 \pm 0.0        & 0.7 \pm 0.0               & 0.7 \pm 0.0            &                    &                           &                        \\
	                           &                                 & TAG         & 0.0 \pm 0.0                   & 0.0 \pm 0.0                 & 0.01 \pm 0.01               & 0.2 \pm 0.0                 & 0.2 \pm 0.0               & 0.2 \pm 0.01           & 0.7 \pm 0.0        & 0.7 \pm 0.0               & 0.7 \pm 0.0            &                    &                           &                        \\
	                           &                                 & TRANSFCONV  & 0.0 \pm 0.0                   & 0.01 \pm 0.01               & 0.02 \pm 0.01               & 0.2 \pm 0.0                 & 0.2 \pm 0.0               & 0.2 \pm 0.01           & 0.7 \pm 0.0        & 0.7 \pm 0.0               & 0.7 \pm 0.0            &                    &                           &                        \\
	                           & \multirow[c]{6}{*}{Topological} & Cell Mp     & 0.0 \pm 0.0                   &                             & 0.0 \pm 0.0                 & 0.03 \pm 0.06               &                           & 0.04 \pm 0.02          & 0.09 \pm 0.21      &                           & 0.3 \pm 0.0            &                    &                           &                        \\
	                           &                                 & Cell Transf & 1.0 \pm 0.0                   &                             & 1.0 \pm 0.0                 & 0.54 \pm 0.0                &                           & 0.54 \pm 0.0           & 0.62 \pm 0.18      &                           & 0.7 \pm 0.0            &                    &                           &                        \\
	                           &                                 & SAN         & 0.0 \pm 0.0                   &                             & 0.01 \pm 0.01               & 0.0 \pm 0.0                 &                           & 0.09 \pm 0.06          & 0.56 \pm 0.31      &                           & 0.41 \pm 0.31          &                    &                           &                        \\
	                           &                                 & SCCN        & 0.07 \pm 0.15                 &                             & 0.03 \pm 0.03               & 0.05 \pm 0.12               &                           & 0.02 \pm 0.01          & 0.1 \pm 0.13       &                           & 0.25 \pm 0.1           &                    &                           &                        \\
	                           &                                 & SCCNN       & 0.0 \pm 0.0                   &                             & 0.0 \pm 0.0                 & 0.12 \pm 0.11               &                           & 0.07 \pm 0.09          & 0.48 \pm 0.32      &                           & 0.24 \pm 0.33          &                    &                           &                        \\
	                           &                                 & SCN         & 0.0 \pm 0.0                   &                             & 0.03 \pm 0.01               & 0.16 \pm 0.09               &                           & 0.13 \pm 0.05          & 0.28 \pm 0.39      &                           & 0.35 \pm 0.16          &                    &                           &                        \\
\end{tabular}
