# Supplementary material for: MANTRA: The Manifold Triangulations Assemblage
Source: arXiv:2410.02392 source file (2025-03-03)
Supplement: Supplementary file 2 [file appendix_betti_auroc_full_stage.tex]

\begin{tabular}{llllllllllll}
{} & {} & {metric} & \multicolumn{9}{c}{AUROC} \\
{} & {} & {task} & \multicolumn{3}{c}{Betti 1} & \multicolumn{3}{c}{Betti 2} & \multicolumn{3}{c}{Betti 3} \\
{} & {} & {transform} & {Degree Transform} & {Degree Transform Onehot} & {Random Node Features} & {Degree Transform} & {Degree Transform Onehot} & {Random Node Features} & {Degree Transform} & {Degree Transform Onehot} & {Random Node Features} \\
{dataset} & {modelclass} & {Model} & {} & {} & {} & {} & {} & {} & {} & {} & {} \\
\multirow[c]{12}{*}{F2D0} & \multirow[c]{5}{*}{Graph} & GAT & 0.5 \pm 0.0 & 0.5 \pm 0.0 & 0.5 \pm 0.0 & 0.5 \pm 0.0 & 0.5 \pm 0.0 & 0.5 \pm 0.0 &  &  &  \\
 &  & GCN & 0.5 \pm 0.0 & 0.5 \pm 0.0 & 0.5 \pm 0.0 & 0.5 \pm 0.0 & 0.5 \pm 0.0 & 0.5 \pm 0.0 &  &  &  \\
 &  & MLP & 0.5 \pm 0.0 & 0.5 \pm 0.0 & 0.5 \pm 0.0 & 0.5 \pm 0.0 & 0.5 \pm 0.0 & 0.5 \pm 0.0 &  &  &  \\
 &  & TAG & 0.5 \pm 0.0 & 0.5 \pm 0.0 & 0.5 \pm 0.0 & 0.5 \pm 0.0 & 0.5 \pm 0.0 & 0.5 \pm 0.0 &  &  &  \\
 &  & TRANSFCONV & 0.5 \pm 0.0 & 0.5 \pm 0.0 & 0.5 \pm 0.0 & 0.5 \pm 0.0 & 0.5 \pm 0.0 & 0.5 \pm 0.0 &  &  &  \\
 & \multirow[c]{7}{*}{Topological} & Cell Mp & 0.62 \pm 0.07 &  & 0.84 \pm 0.0 & 0.49 \pm 0.06 &  & 0.52 \pm 0.02 &  &  &  \\
 &  & Cell Transf & 0.93 \pm 0.01 &  & 0.66 \pm 0.02 & 0.55 \pm 0.0 &  & 0.53 \pm 0.01 &  &  &  \\
 &  & DECT & 0.5 \pm 0.0 & 0.5 \pm 0.0 & 0.5 \pm 0.0 & 0.5 \pm 0.0 & 0.5 \pm 0.0 & 0.5 \pm 0.0 &  &  &  \\
 &  & SAN & 0.55 \pm 0.05 &  & 0.69 \pm 0.06 & 0.52 \pm 0.21 &  & 0.53 \pm 0.01 &  &  &  \\
 &  & SCCN & 0.93 \pm 0.04 &  & 0.78 \pm 0.04 & 0.55 \pm 0.0 &  & 0.53 \pm 0.01 &  &  &  \\
 &  & SCCNN & 0.5 \pm 0.01 &  & 0.5 \pm 0.02 & 0.5 \pm 0.19 &  & 0.52 \pm 0.04 &  &  &  \\
 &  & SCN & 0.56 \pm 0.13 &  & 0.51 \pm 0.03 & 0.63 \pm 0.17 &  & 0.48 \pm 0.07 &  &  &  \\
\multirow[c]{12}{*}{F3D0} & \multirow[c]{5}{*}{Graph} & GAT & 0.23 \pm 0.0 & 0.23 \pm 0.0 & 0.23 \pm 0.0 & 0.12 \pm 0.0 & 0.12 \pm 0.0 & 0.12 \pm 0.0 & 0.14 \pm 0.0 & 0.14 \pm 0.0 & 0.14 \pm 0.0 \\
 &  & GCN & 0.23 \pm 0.0 & 0.23 \pm 0.0 & 0.23 \pm 0.0 & 0.12 \pm 0.0 & 0.12 \pm 0.0 & 0.12 \pm 0.0 & 0.14 \pm 0.0 & 0.14 \pm 0.0 & 0.14 \pm 0.0 \\
 &  & MLP & 0.23 \pm 0.0 & 0.23 \pm 0.0 & 0.23 \pm 0.0 & 0.12 \pm 0.0 & 0.12 \pm 0.0 & 0.12 \pm 0.0 & 0.14 \pm 0.0 & 0.14 \pm 0.0 & 0.14 \pm 0.0 \\
 &  & TAG & 0.23 \pm 0.0 & 0.23 \pm 0.0 & 0.23 \pm 0.0 & 0.12 \pm 0.0 & 0.12 \pm 0.0 & 0.12 \pm 0.0 & 0.14 \pm 0.0 & 0.14 \pm 0.0 & 0.14 \pm 0.0 \\
 &  & TRANSFCONV & 0.23 \pm 0.0 & 0.23 \pm 0.0 & 0.23 \pm 0.0 & 0.12 \pm 0.0 & 0.12 \pm 0.0 & 0.12 \pm 0.0 & 0.14 \pm 0.0 & 0.14 \pm 0.0 & 0.14 \pm 0.0 \\
 & \multirow[c]{7}{*}{Topological} & Cell Mp & 0.23 \pm 0.0 &  & 0.23 \pm 0.0 & 0.12 \pm 0.0 &  & 0.12 \pm 0.0 & 0.14 \pm 0.0 &  & 0.14 \pm 0.0 \\
 &  & Cell Transf & 0.23 \pm 0.0 &  & 0.23 \pm 0.0 & 0.12 \pm 0.0 &  & 0.12 \pm 0.0 & 0.14 \pm 0.0 &  & 0.14 \pm 0.0 \\
 &  & DECT & 0.23 \pm 0.0 & 0.23 \pm 0.0 & 0.23 \pm 0.0 & 0.12 \pm 0.0 & 0.12 \pm 0.0 & 0.12 \pm 0.0 & 0.14 \pm 0.0 & 0.14 \pm 0.0 & 0.14 \pm 0.0 \\
 &  & SAN & 0.17 \pm 0.09 &  & 0.24 \pm 0.01 & 0.12 \pm 0.05 &  & 0.12 \pm 0.0 & 0.19 \pm 0.04 &  & 0.15 \pm 0.01 \\
 &  & SCCN & 0.23 \pm 0.0 &  & 0.23 \pm 0.0 & 0.12 \pm 0.0 &  & 0.12 \pm 0.0 & 0.14 \pm 0.0 &  & 0.14 \pm 0.0 \\
 &  & SCCNN & 0.21 \pm 0.11 &  & 0.2 \pm 0.05 & 0.12 \pm 0.04 &  & 0.11 \pm 0.01 & 0.11 \pm 0.05 &  & 0.13 \pm 0.02 \\
 &  & SCN & 0.2 \pm 0.04 &  & 0.23 \pm 0.0 & 0.15 \pm 0.04 &  & 0.12 \pm 0.0 & 0.11 \pm 0.07 &  & 0.14 \pm 0.02 \\
\multirow[c]{12}{*}{NN2D0} & \multirow[c]{5}{*}{Graph} & GAT & 0.21 \pm 0.0 & 0.21 \pm 0.0 & 0.21 \pm 0.0 & 0.5 \pm 0.0 & 0.5 \pm 0.0 & 0.5 \pm 0.0 &  &  &  \\
 &  & GCN & 0.21 \pm 0.0 & 0.21 \pm 0.0 & 0.21 \pm 0.0 & 0.5 \pm 0.0 & 0.5 \pm 0.0 & 0.5 \pm 0.0 &  &  &  \\
 &  & MLP & 0.21 \pm 0.0 & 0.21 \pm 0.0 & 0.21 \pm 0.0 & 0.5 \pm 0.0 & 0.5 \pm 0.0 & 0.5 \pm 0.0 &  &  &  \\
 &  & TAG & 0.21 \pm 0.0 & 0.21 \pm 0.0 & 0.21 \pm 0.0 & 0.5 \pm 0.0 & 0.5 \pm 0.0 & 0.5 \pm 0.0 &  &  &  \\
 &  & TRANSFCONV & 0.21 \pm 0.0 & 0.21 \pm 0.0 & 0.21 \pm 0.0 & 0.5 \pm 0.0 & 0.5 \pm 0.0 & 0.5 \pm 0.0 &  &  &  \\
 & \multirow[c]{7}{*}{Topological} & Cell Mp & 0.23 \pm 0.01 &  & 0.29 \pm 0.01 & 0.52 \pm 0.04 &  & 0.51 \pm 0.02 &  &  &  \\
 &  & Cell Transf & 0.27 \pm 0.01 &  & 0.21 \pm 0.0 & 0.52 \pm 0.03 &  & 0.5 \pm 0.0 &  &  &  \\
 &  & DECT & 0.21 \pm 0.0 & 0.21 \pm 0.0 & 0.21 \pm 0.0 & 0.5 \pm 0.0 & 0.5 \pm 0.0 & 0.5 \pm 0.0 &  &  &  \\
 &  & SAN & 0.25 \pm 0.01 &  & 0.22 \pm 0.02 & 0.48 \pm 0.04 &  & 0.5 \pm 0.02 &  &  &  \\
 &  & SCCN & 0.29 \pm 0.01 &  & 0.23 \pm 0.01 & 0.52 \pm 0.01 &  & 0.5 \pm 0.02 &  &  &  \\
 &  & SCCNN & 0.2 \pm 0.05 &  & 0.23 \pm 0.03 & 0.49 \pm 0.03 &  & 0.51 \pm 0.02 &  &  &  \\
 &  & SCN & 0.22 \pm 0.0 &  & 0.21 \pm 0.0 & 0.49 \pm 0.02 &  & 0.5 \pm 0.01 &  &  &  \\
\multirow[c]{11}{*}{NN2D1} & \multirow[c]{5}{*}{Graph} & GAT & 0.22 \pm 0.0 & 0.21 \pm 0.0 & 0.21 \pm 0.0 & 0.5 \pm 0.0 & 0.5 \pm 0.0 & 0.5 \pm 0.0 &  &  &  \\
 &  & GCN & 0.22 \pm 0.0 & 0.21 \pm 0.0 & 0.21 \pm 0.0 & 0.5 \pm 0.0 & 0.5 \pm 0.0 & 0.5 \pm 0.0 &  &  &  \\
 &  & MLP & 0.21 \pm 0.01 & 0.21 \pm 0.0 & 0.21 \pm 0.0 & 0.5 \pm 0.0 & 0.5 \pm 0.0 & 0.5 \pm 0.0 &  &  &  \\
 &  & TAG & 0.22 \pm 0.0 & 0.22 \pm 0.0 & 0.22 \pm 0.0 & 0.5 \pm 0.0 & 0.5 \pm 0.0 & 0.5 \pm 0.0 &  &  &  \\
 &  & TRANSFCONV & 0.22 \pm 0.0 & 0.22 \pm 0.0 & 0.22 \pm 0.0 & 0.5 \pm 0.0 & 0.5 \pm 0.0 & 0.5 \pm 0.0 &  &  &  \\
 & \multirow[c]{6}{*}{Topological} & Cell Mp & 0.23 \pm 0.03 &  & 0.26 \pm 0.0 & 0.49 \pm 0.01 &  & 0.49 \pm 0.01 &  &  &  \\
 &  & Cell Transf & 0.23 \pm 0.02 &  & 0.21 \pm 0.0 & 0.5 \pm 0.0 &  & 0.5 \pm 0.0 &  &  &  \\
 &  & SAN & 0.24 \pm 0.01 &  & 0.22 \pm 0.01 & 0.5 \pm 0.0 &  & 0.49 \pm 0.01 &  &  &  \\
 &  & SCCN & 0.27 \pm 0.01 &  & 0.22 \pm 0.01 & 0.52 \pm 0.02 &  & 0.51 \pm 0.01 &  &  &  \\
 &  & SCCNN & 0.21 \pm 0.03 &  & 0.22 \pm 0.02 & 0.5 \pm 0.01 &  & 0.5 \pm 0.01 &  &  &  \\
 &  & SCN & 0.21 \pm 0.0 &  & 0.21 \pm 0.0 & 0.49 \pm 0.02 &  & 0.51 \pm 0.01 &  &  &  \\
\end{tabular}
