# Supplementary material for: MANTRA: The Manifold Triangulations Assemblage
Source: arXiv:2410.02392 source file (2025-03-03)
Supplement: Supplementary file 3 [file appendix_orientability_full_stage.tex]

\begin{tabular}{lllllllll}
{} & {} & {metric} & \multicolumn{3}{c}{AUROC} & \multicolumn{3}{c}{Accuracy} \\
{} & {} & {transform} & {Degree Transform} & {Degree Transform Onehot} & {Random Node Features} & {Degree Transform} & {Degree Transform Onehot} & {Random Node Features} \\
{dataset} & {modelclass} & {Model} & {} & {} & {} & {} & {} & {} \\
\multirow[c]{12}{*}{F2D0} & \multirow[c]{5}{*}{Graph} & GAT & 0.5 \pm 0.0 & 0.5 \pm 0.0 & 0.5 \pm 0.0 & 0.92 \pm 0.0 & 0.92 \pm 0.0 & 0.92 \pm 0.0 \\
 &  & GCN & 0.5 \pm 0.0 & 0.5 \pm 0.0 & 0.5 \pm 0.0 & 0.92 \pm 0.0 & 0.92 \pm 0.0 & 0.92 \pm 0.0 \\
 &  & MLP & 0.5 \pm 0.0 & 0.5 \pm 0.0 & 0.5 \pm 0.0 & 0.92 \pm 0.0 & 0.92 \pm 0.0 & 0.92 \pm 0.0 \\
 &  & TAG & 0.5 \pm 0.0 & 0.5 \pm 0.0 & 0.5 \pm 0.0 & 0.92 \pm 0.0 & 0.92 \pm 0.0 & 0.92 \pm 0.0 \\
 &  & TRANSFCONV & 0.5 \pm 0.0 & 0.5 \pm 0.0 & 0.5 \pm 0.0 & 0.92 \pm 0.0 & 0.92 \pm 0.0 & 0.92 \pm 0.0 \\
 & \multirow[c]{7}{*}{Topological} & Cell Mp & 0.65 \pm 0.07 &  & 0.55 \pm 0.0 & 0.64 \pm 0.26 &  & 0.93 \pm 0.0 \\
 &  & Cell Transf & 0.55 \pm 0.0 &  & 0.5 \pm 0.0 & 0.93 \pm 0.0 &  & 0.92 \pm 0.0 \\
 &  & DECT & 0.5 \pm 0.0 & 0.5 \pm 0.0 & 0.5 \pm 0.0 & 0.92 \pm 0.0 & 0.92 \pm 0.0 & 0.92 \pm 0.0 \\
 &  & SAN & 0.52 \pm 0.03 &  & 0.51 \pm 0.02 & 0.92 \pm 0.0 &  & 0.92 \pm 0.01 \\
 &  & SCCN & 0.55 \pm 0.01 &  & 0.54 \pm 0.01 & 0.93 \pm 0.0 &  & 0.93 \pm 0.0 \\
 &  & SCCNN & 0.55 \pm 0.09 &  & 0.53 \pm 0.02 & 0.87 \pm 0.11 &  & 0.91 \pm 0.01 \\
 &  & SCN & 0.53 \pm 0.04 &  & 0.5 \pm 0.01 & 0.91 \pm 0.02 &  & 0.92 \pm 0.01 \\
\multirow[c]{12}{*}{F3D0} & \multirow[c]{5}{*}{Graph} & GAT & 0.14 \pm 0.0 & 0.14 \pm 0.0 & 0.14 \pm 0.0 & 1.0 \pm 0.0 & 1.0 \pm 0.0 & 1.0 \pm 0.0 \\
 &  & GCN & 0.14 \pm 0.0 & 0.14 \pm 0.0 & 0.14 \pm 0.0 & 1.0 \pm 0.0 & 1.0 \pm 0.0 & 1.0 \pm 0.0 \\
 &  & MLP & 0.14 \pm 0.0 & 0.14 \pm 0.0 & 0.14 \pm 0.0 & 1.0 \pm 0.0 & 1.0 \pm 0.0 & 1.0 \pm 0.0 \\
 &  & TAG & 0.14 \pm 0.0 & 0.14 \pm 0.0 & 0.14 \pm 0.0 & 1.0 \pm 0.0 & 1.0 \pm 0.0 & 1.0 \pm 0.0 \\
 &  & TRANSFCONV & 0.14 \pm 0.0 & 0.14 \pm 0.0 & 0.14 \pm 0.0 & 1.0 \pm 0.0 & 1.0 \pm 0.0 & 1.0 \pm 0.0 \\
 & \multirow[c]{7}{*}{Topological} & Cell Mp & 0.18 \pm 0.04 &  & 0.14 \pm 0.0 & 1.0 \pm 0.0 &  & 1.0 \pm 0.0 \\
 &  & Cell Transf & 0.14 \pm 0.0 &  & 0.14 \pm 0.0 & 1.0 \pm 0.0 &  & 1.0 \pm 0.0 \\
 &  & DECT & 0.14 \pm 0.0 & 0.14 \pm 0.0 & 0.14 \pm 0.0 & 1.0 \pm 0.0 & 1.0 \pm 0.0 & 1.0 \pm 0.0 \\
 &  & SAN & 0.14 \pm 0.0 &  & 0.14 \pm 0.0 & 1.0 \pm 0.0 &  & 1.0 \pm 0.0 \\
 &  & SCCN & 0.14 \pm 0.0 &  & 0.14 \pm 0.0 & 1.0 \pm 0.0 &  & 1.0 \pm 0.0 \\
 &  & SCCNN & 0.14 \pm 0.0 &  & 0.14 \pm 0.0 & 1.0 \pm 0.0 &  & 1.0 \pm 0.0 \\
 &  & SCN & 0.14 \pm 0.0 &  & 0.14 \pm 0.0 & 1.0 \pm 0.0 &  & 1.0 \pm 0.0 \\
\multirow[c]{12}{*}{NN2D0} & \multirow[c]{5}{*}{Graph} & GAT & 0.5 \pm 0.0 & 0.5 \pm 0.0 & 0.5 \pm 0.0 & 0.7 \pm 0.0 & 0.7 \pm 0.0 & 0.7 \pm 0.0 \\
 &  & GCN & 0.5 \pm 0.0 & 0.5 \pm 0.0 & 0.5 \pm 0.0 & 0.7 \pm 0.0 & 0.7 \pm 0.0 & 0.7 \pm 0.0 \\
 &  & MLP & 0.5 \pm 0.0 & 0.5 \pm 0.0 & 0.5 \pm 0.0 & 0.7 \pm 0.0 & 0.7 \pm 0.0 & 0.7 \pm 0.0 \\
 &  & TAG & 0.5 \pm 0.0 & 0.5 \pm 0.0 & 0.5 \pm 0.0 & 0.7 \pm 0.0 & 0.7 \pm 0.0 & 0.7 \pm 0.0 \\
 &  & TRANSFCONV & 0.5 \pm 0.0 & 0.5 \pm 0.0 & 0.5 \pm 0.0 & 0.7 \pm 0.0 & 0.7 \pm 0.0 & 0.7 \pm 0.0 \\
 & \multirow[c]{7}{*}{Topological} & Cell Mp & 0.51 \pm 0.01 &  & 0.5 \pm 0.01 & 0.31 \pm 0.02 &  & 0.7 \pm 0.01 \\
 &  & Cell Transf & 0.52 \pm 0.03 &  & 0.5 \pm 0.0 & 0.72 \pm 0.02 &  & 0.7 \pm 0.0 \\
 &  & DECT & 0.5 \pm 0.0 & 0.5 \pm 0.0 & 0.5 \pm 0.0 & 0.7 \pm 0.0 & 0.7 \pm 0.0 & 0.7 \pm 0.0 \\
 &  & SAN & 0.5 \pm 0.02 &  & 0.51 \pm 0.02 & 0.59 \pm 0.08 &  & 0.6 \pm 0.03 \\
 &  & SCCN & 0.54 \pm 0.01 &  & 0.5 \pm 0.01 & 0.73 \pm 0.0 &  & 0.65 \pm 0.02 \\
 &  & SCCNN & 0.5 \pm 0.01 &  & 0.5 \pm 0.01 & 0.54 \pm 0.23 &  & 0.59 \pm 0.1 \\
 &  & SCN & 0.51 \pm 0.02 &  & 0.51 \pm 0.01 & 0.55 \pm 0.23 &  & 0.61 \pm 0.01 \\
\multirow[c]{11}{*}{NN2D1} & \multirow[c]{5}{*}{Graph} & GAT & 0.5 \pm 0.0 & 0.5 \pm 0.0 & 0.5 \pm 0.0 & 0.7 \pm 0.0 & 0.7 \pm 0.0 & 0.7 \pm 0.0 \\
 &  & GCN & 0.5 \pm 0.0 & 0.5 \pm 0.0 & 0.5 \pm 0.0 & 0.7 \pm 0.0 & 0.7 \pm 0.0 & 0.7 \pm 0.0 \\
 &  & MLP & 0.5 \pm 0.0 & 0.5 \pm 0.0 & 0.5 \pm 0.0 & 0.7 \pm 0.0 & 0.7 \pm 0.0 & 0.7 \pm 0.0 \\
 &  & TAG & 0.5 \pm 0.0 & 0.5 \pm 0.01 & 0.5 \pm 0.0 & 0.64 \pm 0.15 & 0.65 \pm 0.1 & 0.7 \pm 0.0 \\
 &  & TRANSFCONV & 0.5 \pm 0.01 & 0.5 \pm 0.0 & 0.5 \pm 0.0 & 0.6 \pm 0.15 & 0.7 \pm 0.0 & 0.7 \pm 0.0 \\
 & \multirow[c]{6}{*}{Topological} & Cell Mp & 0.5 \pm 0.01 &  & 0.5 \pm 0.0 & 0.38 \pm 0.19 &  & 0.7 \pm 0.0 \\
 &  & Cell Transf & 0.5 \pm 0.0 &  & 0.5 \pm 0.0 & 0.7 \pm 0.0 &  & 0.7 \pm 0.0 \\
 &  & SAN & 0.5 \pm 0.0 &  & 0.5 \pm 0.01 & 0.54 \pm 0.22 &  & 0.49 \pm 0.18 \\
 &  & SCCN & 0.5 \pm 0.0 &  & 0.51 \pm 0.01 & 0.7 \pm 0.0 &  & 0.69 \pm 0.02 \\
 &  & SCCNN & 0.5 \pm 0.0 &  & 0.5 \pm 0.01 & 0.46 \pm 0.22 &  & 0.55 \pm 0.17 \\
 &  & SCN & 0.5 \pm 0.0 &  & 0.5 \pm 0.0 & 0.54 \pm 0.22 &  & 0.68 \pm 0.04 \\
\end{tabular}
