# Supplementary material for: MANTRA: The Manifold Triangulations Assemblage
Source: arXiv:2410.02392 source file (2025-03-03)
Supplement: Supplementary file 9 [file appendix_homeomorphism_full_stage.tex]

\begin{tabular}{lllllllll}
{} & {} & {metric} & \multicolumn{3}{c}{AUROC} & \multicolumn{3}{c}{Accuracy} \\
{} & {} & {transform} & {Degree Transform} & {Degree Transform Onehot} & {Random Node Features} & {Degree Transform} & {Degree Transform Onehot} & {Random Node Features} \\
{dataset} & {modelclass} & {Model} & {} & {} & {} & {} & {} & {} \\
\multirow[c]{12}{*}{F2D0} & \multirow[c]{5}{*}{Graph} & GAT & 0.46 \pm 0.0 & 0.46 \pm 0.0 & 0.47 \pm 0.01 & 0.8 \pm 0.0 & 0.8 \pm 0.0 & 0.8 \pm 0.0 \\
 &  & GCN & 0.46 \pm 0.0 & 0.46 \pm 0.0 & 0.47 \pm 0.01 & 0.8 \pm 0.0 & 0.8 \pm 0.0 & 0.8 \pm 0.0 \\
 &  & MLP & 0.46 \pm 0.0 & 0.46 \pm 0.0 & 0.46 \pm 0.01 & 0.8 \pm 0.0 & 0.8 \pm 0.0 & 0.8 \pm 0.0 \\
 &  & TAG & 0.46 \pm 0.0 & 0.46 \pm 0.0 & 0.46 \pm 0.01 & 0.8 \pm 0.0 & 0.8 \pm 0.0 & 0.8 \pm 0.0 \\
 &  & TRANSFCONV & 0.46 \pm 0.0 & 0.46 \pm 0.0 & 0.46 \pm 0.01 & 0.8 \pm 0.0 & 0.8 \pm 0.0 & 0.8 \pm 0.0 \\
 & \multirow[c]{7}{*}{Topological} & Cell Mp & 0.85 \pm 0.11 &  & 0.89 \pm 0.01 & 0.8 \pm 0.34 &  & 0.94 \pm 0.01 \\
 &  & Cell Transf & 0.91 \pm 0.01 &  & 0.69 \pm 0.15 & 0.94 \pm 0.0 &  & 0.92 \pm 0.01 \\
 &  & DECT & 0.45 \pm 0.0 & 0.45 \pm 0.0 & 0.45 \pm 0.0 & 0.8 \pm 0.0 & 0.8 \pm 0.0 & 0.8 \pm 0.0 \\
 &  & SAN & 0.54 \pm 0.1 &  & 0.67 \pm 0.16 & 0.35 \pm 0.36 &  & 0.72 \pm 0.26 \\
 &  & SCCN & 0.85 \pm 0.08 &  & 0.66 \pm 0.03 & 0.78 \pm 0.35 &  & 0.77 \pm 0.3 \\
 &  & SCCNN & 0.54 \pm 0.1 &  & 0.61 \pm 0.02 & 0.11 \pm 0.0 &  & 0.26 \pm 0.07 \\
 &  & SCN & 0.37 \pm 0.12 &  & 0.5 \pm 0.04 & 0.5 \pm 0.41 &  & 0.73 \pm 0.09 \\
\multirow[c]{12}{*}{NN2D0} & \multirow[c]{5}{*}{Graph} & GAT & 0.48 \pm 0.0 & 0.49 \pm 0.0 & 0.48 \pm 0.0 & 0.54 \pm 0.0 & 0.54 \pm 0.0 & 0.54 \pm 0.0 \\
 &  & GCN & 0.49 \pm 0.0 & 0.48 \pm 0.01 & 0.5 \pm 0.02 & 0.54 \pm 0.0 & 0.54 \pm 0.0 & 0.54 \pm 0.0 \\
 &  & MLP & 0.49 \pm 0.0 & 0.49 \pm 0.0 & 0.48 \pm 0.01 & 0.54 \pm 0.0 & 0.54 \pm 0.0 & 0.54 \pm 0.0 \\
 &  & TAG & 0.49 \pm 0.0 & 0.49 \pm 0.0 & 0.49 \pm 0.01 & 0.54 \pm 0.0 & 0.54 \pm 0.0 & 0.54 \pm 0.0 \\
 &  & TRANSFCONV & 0.49 \pm 0.0 & 0.49 \pm 0.0 & 0.49 \pm 0.01 & 0.54 \pm 0.0 & 0.54 \pm 0.0 & 0.54 \pm 0.0 \\
 & \multirow[c]{7}{*}{Topological} & Cell Mp & 0.63 \pm 0.14 &  & 0.82 \pm 0.0 & 0.19 \pm 0.03 &  & 0.73 \pm 0.0 \\
 &  & Cell Transf & 0.83 \pm 0.01 &  & 0.5 \pm 0.02 & 0.74 \pm 0.0 &  & 0.54 \pm 0.0 \\
 &  & DECT & 0.5 \pm 0.0 & 0.5 \pm 0.0 & 0.48 \pm 0.01 & 0.54 \pm 0.0 & 0.54 \pm 0.0 & 0.54 \pm 0.0 \\
 &  & SAN & 0.49 \pm 0.1 &  & 0.59 \pm 0.1 & 0.54 \pm 0.03 &  & 0.61 \pm 0.03 \\
 &  & SCCN & 0.8 \pm 0.0 &  & 0.65 \pm 0.05 & 0.73 \pm 0.0 &  & 0.57 \pm 0.03 \\
 &  & SCCNN & 0.59 \pm 0.1 &  & 0.52 \pm 0.02 & 0.51 \pm 0.12 &  & 0.55 \pm 0.01 \\
 &  & SCN & 0.53 \pm 0.11 &  & 0.49 \pm 0.06 & 0.3 \pm 0.14 &  & 0.43 \pm 0.03 \\
\multirow[c]{11}{*}{NN2D1} & \multirow[c]{5}{*}{Graph} & GAT & 0.41 \pm 0.03 & 0.53 \pm 0.02 & 0.5 \pm 0.01 & 0.54 \pm 0.0 & 0.54 \pm 0.0 & 0.54 \pm 0.0 \\
 &  & GCN & 0.42 \pm 0.04 & 0.51 \pm 0.04 & 0.5 \pm 0.01 & 0.54 \pm 0.0 & 0.54 \pm 0.0 & 0.54 \pm 0.0 \\
 &  & MLP & 0.43 \pm 0.04 & 0.49 \pm 0.06 & 0.5 \pm 0.01 & 0.54 \pm 0.0 & 0.54 \pm 0.0 & 0.54 \pm 0.0 \\
 &  & TAG & 0.42 \pm 0.04 & 0.5 \pm 0.03 & 0.43 \pm 0.01 & 0.51 \pm 0.09 & 0.33 \pm 0.15 & 0.54 \pm 0.0 \\
 &  & TRANSFCONV & 0.45 \pm 0.03 & 0.42 \pm 0.03 & 0.41 \pm 0.01 & 0.45 \pm 0.13 & 0.54 \pm 0.0 & 0.54 \pm 0.0 \\
 & \multirow[c]{6}{*}{Topological} & Cell Mp & 0.57 \pm 0.06 &  & 0.62 \pm 0.02 & 0.47 \pm 0.17 &  & 0.55 \pm 0.01 \\
 &  & Cell Transf & 0.72 \pm 0.13 &  & 0.49 \pm 0.01 & 0.51 \pm 0.2 &  & 0.54 \pm 0.0 \\
 &  & SAN & 0.49 \pm 0.02 &  & 0.53 \pm 0.04 & 0.48 \pm 0.18 &  & 0.54 \pm 0.0 \\
 &  & SCCN & 0.67 \pm 0.04 &  & 0.53 \pm 0.04 & 0.54 \pm 0.0 &  & 0.54 \pm 0.0 \\
 &  & SCCNN & 0.51 \pm 0.01 &  & 0.51 \pm 0.01 & 0.54 \pm 0.0 &  & 0.54 \pm 0.0 \\
 &  & SCN & 0.51 \pm 0.07 &  & 0.49 \pm 0.04 & 0.35 \pm 0.18 &  & 0.53 \pm 0.03 \\
\end{tabular}
